# Supplementary material for: A Newton Frank-Wolfe Method for Constrained Self-Concordant Minimization
Source: arXiv:2002.07003 source file (2020-02-17)
Supplement: Supplementary file 1 [file refs_supp.tex]

\begin{thebibliography}{28}
\providecommand{\natexlab}[1]{#1}
\providecommand{\url}[1]{\texttt{#1}}
\expandafter\ifx\csname urlstyle\endcsname\relax
  \providecommand{\doi}[1]{doi: #1}\else
  \providecommand{\doi}{doi: \begingroup \urlstyle{rm}\Url}\fi

\bibitem[Bauschke \& Combettes(2017)Bauschke and Combettes]{Bauschke2011}
Bauschke, H.~H. and Combettes, P.
\newblock \emph{Convex analysis and monotone operators theory in {H}ilbert
  spaces}.
\newblock Springer-Verlag, 2nd edition, 2017.


\bibitem[Jaggi(2013)]{Jaggi2013}
Jaggi, M.
\newblock {R}evisiting {F}rank-{W}olfe: {P}rojection-{F}ree {S}parse {C}onvex
  {O}ptimization.
\newblock \emph{JMLR W\&CP}, 28\penalty0 (1):\penalty0 427--435, 2013.


\bibitem[Nesterov(2004)]{Nesterov2004}
Nesterov, Y.
\newblock \emph{{I}ntroductory lectures on convex optimization: {A} basic
  course}, volume~87 of \emph{Applied Optimization}.
\newblock Kluwer Academic Publishers, 2004.

\bibitem[Tran-Dinh et~al.(2019)Tran-Dinh, Sun, and Lu]{TranDinh2016c}
Tran-Dinh, Q., Sun, T., and Lu, S.
\newblock Self-concordant inclusions: A unified framework for path-following
  generalized {N}ewton-type algorithms.
\newblock \emph{Math. Program.}, 177\penalty0 (1--2):\penalty0 173--223, 2019.

\end{thebibliography}
